# Supplementary material for: Prospects for rank-reduced CCSD(T) in the context of high-accuracy thermochemistry
Source: arXiv:2407.19042 ancillary file (2024-07-26)
Supplement: Supplementary file 1 [file supplemental.pdf]

# Prospects for rank-reduced CCSD(T) in the context of high-accuracy thermochemistry: Supplemental Information

Tingting Zhao, James H. Thorpe, and Devin A. Matthews*

*Department of Chemistry, Southern Methodist University, Dallas, TX*

(*Electronic mail: damatthews@smu.edu)

# I. HOOI CONVERGENCE

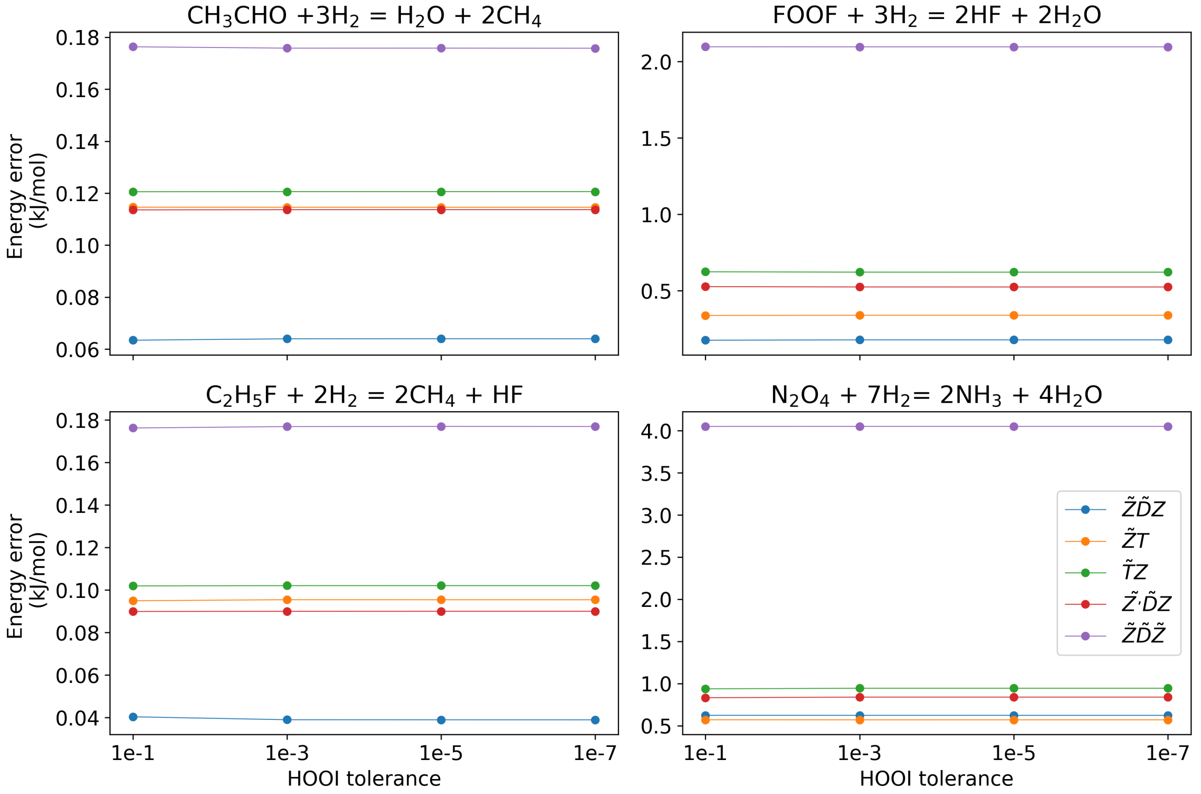


FIG. S1. Absolute errors of AUG-PV{T,Q}Z extrapolated (T) correction energies with respect to the HOOI convergence tolerance. $N_{T_2} = N_{T_3} = 3N_{bas}$.

The HOOI procedure was found to converge very rapidly, and the approximate CCSD(T) energies are highly insensitive to the chosen HOOI convergence criterion (Fig. S1). In some calculations, difficulties were encountered in achieving the requested convergence, typically due to switching of singular vectors between the selected and excluded subsets. In future work, it may be sufficient to simply use a non-iterative estimate of $U$.

# II. COST COMPARISON

To better compare the computational cost of each method, the number of $T_3$ projectors in $n*N_{bas}$ needed to achieve 0.1 kJ/mol accuracy for each reaction species and method were shown in table I.

| Methods | $\tilde{Z}\tilde{D}Z$ | $\tilde{Z}T$ | $\tilde{T}Z$ | $\tilde{Z}'\tilde{D}Z$ | $\tilde{Z}\tilde{D}\tilde{Z}$ |
|---|---|---|---|---|---|
| $SiH_3F$ + $H_2$ -> $SiH_4$ + HF | 2.0 | 2.0 | 1.5 | 1.5 | 2.0 |
| $C_2H_5F + 2H_2 \longrightarrow 2CH_4 + HF$ | 2.0 | 3.0 | 3.5 | 3.0 | 4.5 |
| $2BHF_2 + 3H_2 \longrightarrow B_2H_6 + 2HF$ | 4.5 | 3.0 | 1.5 | 1.5 | 5.5 |
| $CH_3CHO + H_2 \longrightarrow CH_4 + H_2O$ | 2.0 | 3.5 | 3.5 | 3.5 | 4.5 |
| $C_3H_4 + 4H_2 \longrightarrow 3CH_4$ | 2.0 | 3.5 | 3.5 | 3.5 | 3.0 |
| $2BF_3 + 6H_2 \longrightarrow B_2H_6 + 6HF$ | 2.0 | 3.0 | 3.0 | 2.5 | >6 |
| $SiF_4 + 4H_2 \longrightarrow SiH_4 + 4HF$ | 2.0 | 1.5 | 2.0 | 2.0 | >6 |
| $C_6H_6 + 9H_2 \longrightarrow 6CH_4$ | 5.5 | >6 | >6 | >6 | >6 |
| Mean(Single Reference) | 2.75 | 2.79 | 2.64 | 2.5 | 3.9 |
| $N_2 + 3H_2 \longrightarrow 2NH_3$ | 1.5 | 2.0 | 2.0 | 2.0 | 3.0 |
| $2O_2 + H_2 \longrightarrow 2H_2O$ | 2.0 | 3.5 | 3.5 | 3.5 | 4.0 |
| $HCNO + 4H_2 \longrightarrow CH_4 + NH_3 + H_2O$ | 1.0 | 2.5 | 1.5 | 1.5 | 5.5 |
| $HNNN + 4H_2 \longrightarrow 3NH_3$ | 3.5 | 3.5 | 4.0 | 3.5 | 5.5 |
| $SO_3 + 4H_2 \longrightarrow H_2S + 3H_2O$ | 6.0 | 3.5 | 5.0 | 4.5 | >6 |
| $HClO_4 + 4H_2 \longrightarrow HCl + 4H_2O$ | >6 | 4.5 | >6 | >6 | >6 |
| $N_2O_4 + 7H_2 \longrightarrow 2NH_3 + 4H_2O$ | >6 | 6.0 | >6 | >6 | >6 |
| $SF_6 + 4H_2 \longrightarrow 6HF + H_2S$ | >6 | 5.0 | >6 | >6 | >6 |
| Mean(Minor MR) | 2.8 | 3.8 | 3.2 | 3.0 | 4.5 |
| $B_2 + 3H_2 \longrightarrow B_2H_6$ | 1.5 | 1.5 | 2.0 | 2.0 | 2.0 |
| $C_2 + 2H_2 \longrightarrow C_2H_4$ | 2.5 | 2.0 | 2.0 | 2.0 | 3.0 |
| $F_2O + 2H_2 \longrightarrow H_2O + 2HF$ | 6.0 | 4.5 | 6.0 | 6.0 | >6 |
| $O_3 + 3H_2 \longrightarrow 3H_2O$ | 4.5 | 4.0 | 5.0 | 5.0 | >6 |
| $FOOF + 3H_2 \longrightarrow 2H_2O + 2HF$ | 5.5 | 4.5 | 5.5 | 5.5 | >6 |
| $ClF_5 + 3H_2 \longrightarrow 5HF + HCl$ | >6 | 5.5 | >6 | >6 | >6 |
| Mean(Moderate MR) | 4.0 | 3.6 | 4.1 | 4.1 | 2.5 |

TABLE I. $N_{T_3}$ in n*$N_{bas}$ needed to achieve 0.1 kJ/mol for each reaction species and method in aug-cc-PVT,QZ. The species that requires more than 6*$N_{bas}$ projectors were excluded from the mean value calculation as they were not computed, and the n numbers were unknown.

## III. FACTORIZATION OF THE WORKING EQUATIONS

Factorization of the equations for the HOOI procedure, compression of $Z_3/T_3$, and the approximate energy for each approximation scheme were obtained by an in-house contraction search code, with some hand modification as noted. The Einstein summation convention is assumed throughout, and parentheses are used to denote the order of operations.

### A. Explicit formulae and factorization for $Z^{XY}_{ck}$ and $T^{XY}_{ck}$

The factorized equations for the $Z^{XY}_{ck}$ intermediates are given below, along with the associated number of multiplications for each step. Note that a lower-scaling factorization is possible when using rank-reduced amplitudes; the factorization here was chosen so that un-approximated amplitudes $t^{ab}_{ij}$ can also be used easily.

$$\begin{aligned}
Z^{XY}_{ck} &= \frac{1}{6}P(XY)\left\{(C^X_{ai}(E1^{JY}_{ai}+E2^{JY}_{ai}))B^J_{ck}\right. && 2N_{DF}N^2_{T_3}vo \\
&\quad + C^X_{ak}D1^Y_{ca} - C^X_{ci}D2^Y_{ik} && N^2_{T_3}Nvo \\
&\quad \left. + \tilde{t}^{bc}_{ik}(U^Y_{ai}D1^Z_{ab} - U^Y_{bj}D2^Z_{ij})\right\} && N^2_{T_3}v^2o^2 + N^2_{T_3}Nvo && (1) \\
C^X_{ai} &= V^W_{ai}(T^{VW}(V^V_{bj}U^X_{bj})) && 2N_{T_2}N_{T_3}vo + N^2_{T_2}N_{T_3} && (2) \\
D1^X_{ab} &= B^J_{ab}(B^J_{ck}U^X_{ck}) && N_{DF}N_{T_3}Nv && (3) \\
D2^X_{ij} &= B^J_{ij}(B^J_{ck}U^X_{ck}) && N_{DF}N_{T_3}No && (4) \\
E1^{JX}_{ai} &= B^J_{ab}U^X_{bi} && N_{DF}N_{T_3}v^2o && (5) \\
E2^{JX}_{ai} &= -B^J_{ji}U^X_{aj} && N_{DF}N_{T_3}vo^2 && (6) \\
\tilde{t}^{ab}_{ij} &= V^V_{ai}T^{VW}V^W_{bj} && N_{T_2}v^2o^2 + N^2_{T_2}vo, && (7)
\end{aligned}$$

where the permutation operator $P(XY) = (XY) + (YX)$. The construction of $T^{XY}_{ck}$ uses an identical factorization apart from the insertion of the Laplace factors $\tau^g_a$ and $\tau^g_i$ and the summation of all terms over $g$. Laplace factors must be inserted for every molecular orbital index of $U$, and also for the external indices $ck$ in (1).

## B. Explicit formulae and factorization for $Z^{XYZ}$

The explicit formulae and factorization for the fourth-order E4T portion of $Z^{XYZ}$ are shown as follows ( including the number of multiplications required for each step)

$$(Z^{XYZ})^{[4]} = P(XYZ)\left\{C^X_{ai}(E1^{JY}_{ai} + E2^{JY}_{ai})F^{JZ}\right\} \qquad N_{DF}N^2_{T_3}vo + N_{DF}N^3_{T_3} \tag{8}$$

$$F^{JX} = B^J_{ai}U^X_{ai} \qquad N_{DF}N_{T_3}vo \tag{9}$$

where the permutation operator $P(XYZ) = (XYZ) + (XZY) + (YXZ) + (YZX) + (ZXY) + (ZYX)$. To construct $T^{XYZ}$ via Laplace denominators, the Laplace factors $\tau^g_a$ and $\tau^g_i$ must be again included for each molecular orbital index of $U$, followed by a summation over $g$. The fifth-order term E5ST is always included through the top $Z_3$ or $T_3$ fragment in our calculations, and is thus always included in the Tucker-3 compression. We do *not* include this term in the HOOI procedure, and limited testing shows a negligible effect on the computed projectors. The explicit formula and factorization, including number of multiplications, for this term is

$$(Z^{XYZ})^{[5]} = \frac{1}{2}P(XYZ)\left\{G^X F^{JY} F^{JZ}\right\} \qquad (N_{DF} + N_{T_3})N^2_{T_3} \tag{10}$$

$$G^X = U^X_{ai}t^a_i \qquad N_{T_3}vo \tag{11}$$

## C. Explicit formulae and factorization for approximate (T) energy: $\tilde{Z}\tilde{D}\tilde{Z}$

The explicit formulae and factorization for $E^{\tilde{Z}\tilde{D}\tilde{Z}}_{(T)}$ are given below. $E^5$ST is included in the top $\tilde{Z}_3\tilde{D}_3 = \tilde{T}_3$ fragment in this approximation scheme.

$$\begin{aligned} E^{\tilde{Z}\tilde{D}\tilde{Z}}_{(T)} =& \frac{1}{3}\{4\,T^{XYZ}U^X_{ai}U^Y_{bj}U^Z_{ck}U^A_{ai}U^B_{bj}U^C_{ck}Z^{ABC} \\ & -6\,T^{XYZ}U^X_{ai}U^Y_{bj}U^Z_{ck}U^A_{ak}U^B_{bj}U^C_{ci}Z^{ABC} \\ & +2\,T^{XYZ}U^X_{ai}U^Y_{bj}U^Z_{ck}U^A_{ak}U^B_{bi}U^C_{cj}Z^{ABC}\} \end{aligned} \tag{12}$$

$$\begin{aligned} =& \frac{1}{3}\{4\,T^{XYZ}Z^{XYZ} && N^3_{T_3} \\ & -J1^{YA}_{ci}(6I2^{AB}_{ci}\delta_{YB} - 2J2^{YA}_{ci})\} && N^2_{T_3}vo \end{aligned} \tag{13}$$

$$H^{XA}_{ij} = U^X_{ai}U^Y_{aj} \qquad N^2_{T_3}vo^2 \tag{14}$$

$$I1^{XY}_{ck} = U^Z_{ck}T^{XYZ} \qquad N^3_{T_3}vo \tag{15}$$

$$I2^{AB}_{ci} = U^C_{ci}Z^{ABC} \qquad N^3_{T_3}vo \tag{16}$$

$$J1^{YA}_{ci} = H^{XA}_{ik}I1^{XY}_{ck} \qquad N^3_{T_3}vo^2 \tag{17}$$

$$J2^{YA}_{ci} = H^{YB}_{ji} I2^{AB}_{cj} \qquad N^3_{T_3} vo^2, \tag{18}$$

where $U^X_{ai} U^A_{ai} = \delta_{XA}$.

## D. Explicit formulae and factorization for approximate (T) energy: other schemes

The explicit formulae and factorization for the remaining approximation schemes: $\tilde{T}Z$, $\tilde{Z}\tilde{D}Z$, and $\tilde{Z}'\tilde{D}Z$ share a common structure, and the equations for $\tilde{T}Z$ are given below as an exemple. For $\tilde{Z}T$, there is in addition a sum over the Laplace quadrature points $g$, and Laplace factors $\tau^g_a$ and $\tau^g_i$ must be inserted for each MO $abcijk$ (which can be easily accomplished by pre-applying the factors to the $U$ projectors). Note that the equations are factored in such a way as to allow the exact $T_2$ to be easily used if desired, although for the (T) energy little-to-no cost reduction is possible by assuming rank-reduced $T_2$ amplitudes.

$$\begin{aligned}
E^{\tilde{T}Z}_{(T)} =& \{4\,T^{XYZ} U^X_{ai} U^Y_{bj} U^Z_{ck} (\tilde{t}^{ad}_{ij} B^J_{bd} - \tilde{t}^{ab}_{il} B^J_{lj}) B^J_{ck} \\
& - 2\,T^{XYZ} U^X_{aj} U^Y_{bi} U^Z_{ck} (\tilde{t}^{ad}_{ji} B^J_{bd} - \tilde{t}^{ab}_{jl} B^J_{li}) B^J_{ck} \\
& - 2\,T^{XYZ} U^X_{ai} U^Y_{bj} U^Z_{ck} (\tilde{t}^{ad}_{kj} B^J_{bd} - \tilde{t}^{ab}_{kl} B^J_{lj}) B^J_{ci} \\
& + T^{XYZ} U^X_{ai} U^Y_{bj} U^Z_{ck} (\tilde{t}^{ad}_{jk} B^J_{bd} - \tilde{t}^{ab}_{jl} B^J_{lk}) B^J_{ci} \\
& - T^{XYZ} U^X_{ai} U^Y_{bj} U^Z_{ck} (\tilde{t}^{ad}_{ik} B^J_{bd} - \tilde{t}^{ab}_{il} B^J_{lk}) B^J_{cj} \\
& + T^{XYZ} U^X_{ai} U^Y_{bj} U^Z_{ck} (\tilde{t}^{ad}_{ki} B^J_{bd} - \tilde{t}^{ab}_{kl} B^J_{li}) B^J_{cj}\}
\end{aligned} \tag{19}$$

$$\begin{aligned}
=& \{2\,(\tilde{C}^X_{dl}(E1^{JY}_{dl} + E2^{JY}_{dl}) T^{XYZ}) F^{JZ} && N_{DF} N^2_{T_3} vo + N_{DF} N^3_{T_3} + N_{DF} N_{T_3} \\
& - (2\tilde{t}^{ad}_{kl} - \tilde{t}^{ad}_{lk})(E1^{JY}_{dl} + E2^{JY}_{dl})(E3^{JZ}_{ik} I1^{YZ}_{ai}) && N_{DF} N^2_{T_3} vo^2 + N_{DF} N_{T_3} v^2 o^2 + v^2 o^2 \\
& - \tilde{C}^X_{dl} K^X_{dl}\} && N_{T_3} vo
\end{aligned} \tag{20}$$

$$\tilde{C}^X_{ai} = (2\tilde{t}^{ab}_{ij} - \tilde{t}^{ab}_{ji}) U^X_{bj} \qquad N_{T_3} v^2 o^2 \tag{21}$$

$$E3^{JZ}_{ik} = B^J_{ci} U^Z_{ck} \qquad N_{DF} N_{T_3} vo^2 \tag{22}$$

$$K^X_{dl} = (D1^Y_{cd} U^Z_{cl} - D2^Y_{lk} U^Z_{dk}) T^{XYZ} \qquad N^2_{T_3} Nvo + N^3_{T_3} vo \tag{23}$$
